# Supplementary material for: Neural Network based Explicit Mixture Models and Expectation-maximization based Learning
Source: arXiv:1907.13432 source file (2020-05-24)
Supplement: Supplementary file 2 [file emgm-sm.tex]

% Graphic for TeX using PGF
% Title: /home/dong/Documents/draft/increamentalOT/images/diagram/emgm-sm.dia
% Creator: Dia v0.97.3
% CreationDate: Fri Jan  4 16:26:51 2019
% For: dong
% \usepackage{tikz}
% The following commands are not supported in PSTricks at present
% We define them conditionally, so when they are implemented,
% this pgf file will use them.
\ifx\du\undefined
  \newlength{\du}
\fi
\setlength{\du}{15\unitlength}
\begin{tikzpicture}[scale=0.9]
\pgftransformxscale{1.000000}
\pgftransformyscale{-1.000000}
\definecolor{dialinecolor}{rgb}{0.000000, 0.000000, 0.000000}
\pgfsetstrokecolor{dialinecolor}
\definecolor{dialinecolor}{rgb}{1.000000, 1.000000, 1.000000}
\pgfsetfillcolor{dialinecolor}
\definecolor{dialinecolor}{rgb}{1.000000, 1.000000, 1.000000}
\pgfsetfillcolor{dialinecolor}
\pgfpathellipse{\pgfpoint{6.322568\du}{12.347997\du}}{\pgfpoint{1.377568\du}{0\du}}{\pgfpoint{0\du}{0.758267\du}}
\pgfusepath{fill}
\pgfsetlinewidth{0.100000\du}
\pgfsetdash{}{0pt}
\pgfsetdash{}{0pt}
\definecolor{dialinecolor}{rgb}{0.000000, 0.000000, 0.000000}
\pgfsetstrokecolor{dialinecolor}
\pgfpathellipse{\pgfpoint{6.322568\du}{12.347997\du}}{\pgfpoint{1.377568\du}{0\du}}{\pgfpoint{0\du}{0.758267\du}}
\pgfusepath{stroke}
% setfont left to latex
\definecolor{dialinecolor}{rgb}{0.000000, 0.000000, 0.000000}
\pgfsetstrokecolor{dialinecolor}
\node[anchor=west] at (5.139574\du,12.464986\du){$\bm{z}\sim p_1$};
\pgfsetlinewidth{0.100000\du}
\pgfsetdash{{\pgflinewidth}{0.200000\du}}{0cm}
\pgfsetdash{{\pgflinewidth}{0.200000\du}}{0cm}

\pgfsetbuttcap
{
\definecolor{dialinecolor}{rgb}{0.000000, 0.000000, 0.000000}
\pgfsetfillcolor{dialinecolor}
% was here!!!
\pgfsetarrowsend{latex}
\pgfsetarrowsstart{latex}

\definecolor{dialinecolor}{rgb}{0.000000, 0.000000, 0.000000}
\pgfsetstrokecolor{dialinecolor}
\draw (7.997078\du,12.525883\du)--(12.009693\du,15.126247\du);
}
\pgfsetlinewidth{0.100000\du}

\pgfsetdash{{\pgflinewidth}{0.200000\du}}{0cm}
\pgfsetdash{{\pgflinewidth}{0.200000\du}}{0cm}

\pgfsetbuttcap
{
\definecolor{dialinecolor}{rgb}{0.000000, 0.000000, 0.000000}
\pgfsetfillcolor{dialinecolor}
% was here!!!
\pgfsetarrowsend{latex}
\pgfsetarrowsstart{latex}

\definecolor{dialinecolor}{rgb}{0.000000, 0.000000, 0.000000}
\pgfsetstrokecolor{dialinecolor}
\draw (7.897106\du,19.603640\du)--(12.025903\du,16.520345\du);
}
\pgfsetlinewidth{0.100000\du}
\pgfsetdash{}{0pt}
\pgfsetdash{}{0pt}
\pgfsetbuttcap
{
\definecolor{dialinecolor}{rgb}{0.000000, 0.000000, 0.000000}
\pgfsetfillcolor{dialinecolor}
% was here!!!
\pgfsetarrowsend{latex}
\pgfsetarrowsstart{latex}
\definecolor{dialinecolor}{rgb}{0.000000, 0.000000, 0.000000}
\pgfsetstrokecolor{dialinecolor}
\draw (7.892240\du,15.012774\du)--(12.025903\du,15.952980\du);
}
\definecolor{dialinecolor}{rgb}{1.000000, 1.000000, 1.000000}
\pgfsetfillcolor{dialinecolor}
\pgfpathellipse{\pgfpoint{17.144180\du}{15.849715\du}}{\pgfpoint{1.377568\du}{0\du}}{\pgfpoint{0\du}{0.758267\du}}
\pgfusepath{fill}
\pgfsetlinewidth{0.100000\du}
\pgfsetdash{}{0pt}
\pgfsetdash{}{0pt}
\definecolor{dialinecolor}{rgb}{0.000000, 0.000000, 0.000000}
\pgfsetstrokecolor{dialinecolor}
\pgfpathellipse{\pgfpoint{17.144180\du}{15.849715\du}}{\pgfpoint{1.377568\du}{0\du}}{\pgfpoint{0\du}{0.758267\du}}
\pgfusepath{stroke}
% setfont left to latex
\definecolor{dialinecolor}{rgb}{0.000000, 0.000000, 0.000000}
\pgfsetstrokecolor{dialinecolor}
\node[anchor=west] at (15.65\du,15.8\du){$\bm{x}\sim \widetilde{P}_g$};
\definecolor{dialinecolor}{rgb}{1.000000, 1.000000, 1.000000}
\pgfsetfillcolor{dialinecolor}
\pgfpathellipse{\pgfpoint{6.386600\du}{14.871153\du}}{\pgfpoint{1.377568\du}{0\du}}{\pgfpoint{0\du}{0.758267\du}}
\pgfusepath{fill}
\pgfsetlinewidth{0.100000\du}
\pgfsetdash{}{0pt}
\pgfsetdash{}{0pt}
\definecolor{dialinecolor}{rgb}{0.000000, 0.000000, 0.000000}
\pgfsetstrokecolor{dialinecolor}
\pgfpathellipse{\pgfpoint{6.386600\du}{14.871153\du}}{\pgfpoint{1.377568\du}{0\du}}{\pgfpoint{0\du}{0.758267\du}}
\pgfusepath{stroke}
% setfont left to latex
\definecolor{dialinecolor}{rgb}{0.000000, 0.000000, 0.000000}
\pgfsetstrokecolor{dialinecolor}
\node[anchor=west] at (5.203606\du,14.988141\du){$\bm{z}\sim p_2$};
% setfont left to latex
\definecolor{dialinecolor}{rgb}{0.000000, 0.000000, 0.000000}
\pgfsetstrokecolor{dialinecolor}
\node[anchor=west] at (6. \du,16.029692\du){.};
\node[anchor=west] at (6. \du,17.029692\du){.};
\node[anchor=west] at (6. \du,18.029692\du){.};

\definecolor{dialinecolor}{rgb}{1.000000, 1.000000, 1.000000}
\pgfsetfillcolor{dialinecolor}
\pgfpathellipse{\pgfpoint{6.434421\du}{19.469245\du}}{\pgfpoint{1.377568\du}{0\du}}{\pgfpoint{0\du}{0.758267\du}}
\pgfusepath{fill}
\pgfsetlinewidth{0.100000\du}
\pgfsetdash{}{0pt}
\pgfsetdash{}{0pt}
\definecolor{dialinecolor}{rgb}{0.000000, 0.000000, 0.000000}
\pgfsetstrokecolor{dialinecolor}
\pgfpathellipse{\pgfpoint{6.434421\du}{19.469245\du}}{\pgfpoint{1.377568\du}{0\du}}{\pgfpoint{0\du}{0.758267\du}}
\pgfusepath{stroke}
% setfont left to latex
\definecolor{dialinecolor}{rgb}{0.000000, 0.000000, 0.000000}
\pgfsetstrokecolor{dialinecolor}
\node[anchor=west] at (5.051426\du,19.586233\du){$\bm{z}\sim p_K$};
\pgfsetlinewidth{0.100000\du}
\pgfsetdash{}{0pt}
\pgfsetdash{}{0pt}
\pgfsetbuttcap
\pgfsetmiterjoin
\pgfsetlinewidth{0.100000\du}
\pgfsetbuttcap
\pgfsetmiterjoin
\pgfsetdash{}{0pt}
\definecolor{dialinecolor}{rgb}{1.000000, 1.000000, 1.000000}
\pgfsetfillcolor{dialinecolor}
\fill (12.333649\du,15.197321\du)--(12.333649\du,16.513191\du)--(13.607072\du,16.513191\du)--(13.607072\du,15.197321\du)--cycle;
\definecolor{dialinecolor}{rgb}{0.000000, 0.000000, 0.000000}
\pgfsetstrokecolor{dialinecolor}
\draw (12.333649\du,15.197321\du)--(12.333649\du,16.513191\du)--(13.607072\du,16.513191\du)--(13.607072\du,15.197321\du)--cycle;
\pgfsetbuttcap
\pgfsetmiterjoin
\pgfsetdash{}{0pt}
\definecolor{dialinecolor}{rgb}{0.000000, 0.000000, 0.000000}
\pgfsetstrokecolor{dialinecolor}
\draw (12.333649\du,15.197321\du)--(12.333649\du,16.513191\du)--(13.607072\du,16.513191\du)--(13.607072\du,15.197321\du)--cycle;
% setfont left to latex
\definecolor{dialinecolor}{rgb}{0.000000, 0.000000, 0.000000}
\pgfsetstrokecolor{dialinecolor}
\node[anchor=west] at (12.521331\du,15.936846\du){$g$};
\pgfsetlinewidth{0.100000\du}
\pgfsetdash{}{0pt}
\pgfsetdash{}{0pt}
\pgfsetbuttcap
{
\definecolor{dialinecolor}{rgb}{0.000000, 0.000000, 0.000000}
\pgfsetfillcolor{dialinecolor}
% was here!!!
\pgfsetarrowsend{latex}
\pgfsetarrowsstart{latex}
\definecolor{dialinecolor}{rgb}{0.000000, 0.000000, 0.000000}

\pgfsetstrokecolor{dialinecolor}
\draw (13.707737\du,15.920559\du)--(15.625145\du,15.909711\du);
}
% setfont left to latex
\definecolor{dialinecolor}{rgb}{0.000000, 0.000000, 0.000000}
\pgfsetstrokecolor{dialinecolor}
\node[anchor=west] at (8.40\du,13.64363\du){$\pi_1$};
% setfont left to latex
\definecolor{dialinecolor}{rgb}{0.000000, 0.000000, 0.000000}
\pgfsetstrokecolor{dialinecolor}
\node[anchor=west] at (8.40\du,15.9\du){$\pi_2$};
% setfont left to latex
\definecolor{dialinecolor}{rgb}{0.000000, 0.000000, 0.000000}
\pgfsetstrokecolor{dialinecolor}
\node[anchor=west] at (8.40\du,19.4\du){$\pi_K$};
\end{tikzpicture}

%%% Local Variables:
%%% mode: latex
%%% TeX-master: "../../naive_mix_icml"
%%% End:
